# Supplementary material for: Approximations to the exact exchange potential: KLI versus semilocal
Source: arXiv:1608.08415 ancillary file (2016-08-30)
Supplement: Supplementary file 1 [file Supplemental_Material.pdf]

# Supplemental Material for
# Approximations to the exact exchange potential: KLI versus semilocal

Fabien Tran and Peter Blaha
*Institute of Materials Chemistry, Vienna University of Technology,*
*Getreidemarkt 9/165-TC, A-1060 Vienna, Austria*

Markus Betzinger and Stefan Blügel
*Peter-Grünberg Institut and Institute for Advanced Simulation,*
*Forschungszentrum Jülich and JARA, D-52425 Jülich, Germany*

TABLE S1. The space group and geometrical parameters of the solids considered in this work. The lattice parameters are in Å and the internal parameters are in internal units. For MnO and NiO, the antiferromagnetic order leads to a lowering of the symmetry (second indicated space group). The last column shows the electrons that were considered as core electrons, for which a fully relativistic treatment (i.e., spin-orbit coupling included) is used.

| Solid | Space group | Geometrical parameters | Core states |
|---|---|---|---|
| Ne | $Fm\bar{3}m$ | $a = 4.470$ | $1s$ |
| C | $Fd\bar{3}m$ | $a = 3.568$ | $1s$ |
| Si | $Fd\bar{3}m$ | $a = 5.429$ | $1s$ |
| Ge | $Fd\bar{3}m$ | $a = 5.652$ | [Ne] |
| BN | $F\bar{4}3m$ | $a = 3.616$ | B: $1s$; N: $1s$ |
| LiH | $Fm\bar{3}m$ | $a = 4.084$ | |
| LiF | $Fm\bar{3}m$ | $a = 4.010$ | F: $1s$ |
| LiCl | $Fm\bar{3}m$ | $a = 5.106$ | Cl: [Ne] |
| BeO | $P6_3mc$ | $a = 2.694$, $c = 4.384$, $z_{\rm O} = 0.378$ | Be: $1s$; O: $1s$ |
| MgO | $Fm\bar{3}m$ | $a = 4.228$ | Mg: $1s$; O: $1s$ |
| BaO | $Fm\bar{3}m$ | $a = 5.523$ | Ba: [Kr]; O: $1s$ |
| MnO | $Fm\bar{3}m$, $R\bar{3}m$ | $a = 4.445$ | Mn: [Ne]; O: $1s$ |
| NiO | $Fm\bar{3}m$, $R\bar{3}m$ | $a = 4.171$ | Ni: [Ne]; O: $1s$ |
| $Cu_2O$ | $Pn\bar{3}m$ | $a = 4.267$ | Cu: [Ne]; O: $1s$ |
| ZnO | $P6_3mc$ | $a = 3.258$, $c = 5.220$, $z_{\rm O} = 0.382$ | Zn: [Ne]$3s$; O: $1s$ |
| $CeO_2$ | $Fm\bar{3}m$ | $a = 5.411$ | Ce: [Kr]$4d$; O: $1s$ |

## I. SOLIDS

The solids considered in this work for the comparison of exchange potentials are listed in Table S1 along with their space group, geometrical parameters, and the core states.

## II. DETAILS OF THE EXX-KLI POTENTIAL FOR THE LAPW BASIS SET

In a periodic solid, the spin-$\sigma$ electrons are represented by Bloch orbitals $\psi_{n\boldsymbol{k}}^{\sigma}$, where $n$ is the band index and $\boldsymbol{k}$ is a wave vector of the first Brillouin zone. However, since the deep-lying core electrons are well localized around the nuclei and do not hybridize they can be treated separately from the valence electrons and with atomic-like orbitals $\psi_{n_c\ell_c m_c}^{\alpha\sigma}$, where $\alpha$ is the atom index, and $n_c$, $\ell_c$, and $m_c$ are the principal, azimuthal, and magnetic quantum numbers, respectively. The basic formulas of the EXX-KLI potential when such a different treatment for the valence (v) and core (c) electrons is done (like in the LAPW basis set[1–3]) are given below. In the following equations, $w_{n\boldsymbol{k}}^{\sigma}$ is the product of the $\boldsymbol{k}$-point weight and the occupation number, $\Omega$ denotes the unit cell, and $S_\alpha$ the LAPW atomic sphere surrouding the atom $\alpha$.

The EXX-KLI potential, Eq. (2), is given by

$$v_{{\rm x},\sigma}^{\text{EXX-KLI}}(\boldsymbol{r}) = v_{{\rm x},\sigma}^{\rm S}(\boldsymbol{r}) + v_{{\rm x},\sigma}^{\rm KLI,1}(\boldsymbol{r}) + v_{{\rm x},\sigma}^{\rm KLI,2}(\boldsymbol{r}). \tag{S1}$$

$v_{{\rm x},\sigma}^{\rm S}$ is the Slater potential which is given by

$$v_{{\rm x},\sigma}^{\rm S}(\boldsymbol{r}) = v_{{\rm x},\sigma}^{\rm S,vv}(\boldsymbol{r}) + v_{{\rm x},\sigma}^{\rm S,vc}(\boldsymbol{r}) + v_{{\rm x},\sigma}^{\rm S,cv}(\boldsymbol{r}) + v_{{\rm x},\sigma}^{\rm S,cc}(\boldsymbol{r}), \tag{S2}$$

where

$$v_{{\rm x},\sigma}^{\rm S,vv}(\boldsymbol{r}) = -\frac{1}{\rho_\sigma(\boldsymbol{r})}\sum_{n,\boldsymbol{k}}\sum_{n',\boldsymbol{k}'} w_{n\boldsymbol{k}}^{\sigma} w_{n'\boldsymbol{k}'}^{\sigma} \psi_{n\boldsymbol{k}}^{\sigma*}(\boldsymbol{r})\psi_{n'\boldsymbol{k}'}^{\sigma}(\boldsymbol{r}) \int\limits_{\rm crystal} \frac{\psi_{n'\boldsymbol{k}'}^{\sigma*}(\boldsymbol{r}')\psi_{n\boldsymbol{k}}^{\sigma}(\boldsymbol{r}')}{|\boldsymbol{r}-\boldsymbol{r}'|} d^3r', \tag{S3}$$

$$v_{{\rm x},\sigma}^{\rm S,vc}(\boldsymbol{r}) = -\frac{1}{\rho_\sigma(\boldsymbol{r})}\sum_{n,\boldsymbol{k}}\sum_{\alpha}^{\rm cell}\sum_{n_c,\ell_c,m_c} w_{n\boldsymbol{k}}^{\sigma} \psi_{n\boldsymbol{k}}^{\sigma*}(\boldsymbol{r})\psi_{n_c\ell_c m_c}^{\alpha\sigma}(\boldsymbol{r}) \int\limits_{S_\alpha} \frac{\psi_{n_c\ell_c m_c}^{\alpha\sigma*}(\boldsymbol{r}')\psi_{n\boldsymbol{k}}^{\sigma}(\boldsymbol{r}')}{|\boldsymbol{r}-\boldsymbol{r}'|} d^3r', \tag{S4}$$

$$v_{{\rm x},\sigma}^{\rm S,cv}(\boldsymbol{r}) = -\frac{1}{\rho_\sigma(\boldsymbol{r})}\sum_{\alpha}^{\rm cell}\sum_{n_c,\ell_c,m_c}\sum_{n,\boldsymbol{k}} w_{n\boldsymbol{k}}^{\sigma} \psi_{n_c\ell_c m_c}^{\alpha\sigma*}(\boldsymbol{r})\psi_{n\boldsymbol{k}}^{\sigma}(\boldsymbol{r}) \int\limits_{S_\alpha} \frac{\psi_{n\boldsymbol{k}}^{\sigma*}(\boldsymbol{r}')\psi_{n_c\ell_c m_c}^{\alpha\sigma}(\boldsymbol{r}')}{|\boldsymbol{r}-\boldsymbol{r}'|} d^3r', \tag{S5}$$

$$v_{\mathrm{x},\sigma}^{\mathrm{S,cc}}(\boldsymbol{r}) = -\frac{1}{\rho_\sigma(\boldsymbol{r})}\sum_{\alpha}^{\mathrm{cell}}\sum_{n_c,\ell_c,m_c}\sum_{n_c',\ell_c',m_c'}\psi_{n_c\ell_cm_c}^{\alpha\sigma*}(\boldsymbol{r})\psi_{n_c'\ell_c'm_c'}^{\alpha\sigma}(\boldsymbol{r})\int\limits_{S_\alpha}\frac{\psi_{n_c'\ell_c'm_c'}^{\alpha\sigma*}(\boldsymbol{r}')\psi_{n_c\ell_cm_c}^{\alpha\sigma}(\boldsymbol{r}')}{|\boldsymbol{r}-\boldsymbol{r}'|}d^3r'. \tag{S6}$$

The second term in Eq. (S1), which involves the EXX-KLI potential itself, is given by

$$v_{\mathrm{x},\sigma}^{\mathrm{KLI,1}}(\boldsymbol{r}) = v_{\mathrm{x},\sigma}^{\mathrm{KLI,1,v}}(\boldsymbol{r}) + v_{\mathrm{x},\sigma}^{\mathrm{KLI,1,c}}(\boldsymbol{r}), \tag{S7}$$

where

$$v_{\mathrm{x},\sigma}^{\mathrm{KLI,1,v}}(\boldsymbol{r}) = \frac{1}{\rho_\sigma(\boldsymbol{r})}\sum_{n,\boldsymbol{k}}w_{n\boldsymbol{k}}^{\sigma}\left|\psi_{n\boldsymbol{k}}^{\sigma}(\boldsymbol{r})\right|^2\int\limits_{\Omega}\psi_{n\boldsymbol{k}}^{\sigma*}(\boldsymbol{r}')v_{\mathrm{x},\sigma}^{\text{EXX-KLI}}(\boldsymbol{r}')\psi_{n\boldsymbol{k}}^{\sigma}(\boldsymbol{r}')d^3r', \tag{S8}$$

$$v_{\mathrm{x},\sigma}^{\mathrm{KLI,1,c}}(\boldsymbol{r}) = \frac{1}{\rho_\sigma(\boldsymbol{r})}\sum_{\alpha}^{\mathrm{cell}}\sum_{n_c,\ell_c,m_c}\left|\psi_{n_c\ell_cm_c}^{\alpha\sigma}(\boldsymbol{r})\right|^2\int\limits_{S_\alpha}\psi_{n_c\ell_cm_c}^{\alpha\sigma*}(\boldsymbol{r}')v_{\mathrm{x},\sigma}^{\text{EXX-KLI}}(\boldsymbol{r}')\psi_{n_c\ell_cm_c}^{\alpha\sigma}(\boldsymbol{r}')d^3r', \tag{S9}$$

while the third term in Eq. (S1) involving the Hartree-Fock operator is given by

$$v_{\mathrm{x},\sigma}^{\mathrm{KLI,2}}(\boldsymbol{r}) = v_{\mathrm{x},\sigma}^{\mathrm{KLI,2,vv}}(\boldsymbol{r}) + v_{\mathrm{x},\sigma}^{\mathrm{KLI,2,vc}}(\boldsymbol{r}) + v_{\mathrm{x},\sigma}^{\mathrm{KLI,2,cv}}(\boldsymbol{r}) + v_{\mathrm{x},\sigma}^{\mathrm{KLI,2,cc}}(\boldsymbol{r}), \tag{S10}$$

where

$$v_{\mathrm{x},\sigma}^{\mathrm{KLI,2,vv}}(\boldsymbol{r}) = \frac{1}{\rho_\sigma(\boldsymbol{r})}\sum_{n,\boldsymbol{k}}\sum_{n',\boldsymbol{k}'}w_{n\boldsymbol{k}}^{\sigma}w_{n'\boldsymbol{k}'}^{\sigma}\left|\psi_{n\boldsymbol{k}}^{\sigma}(\boldsymbol{r})\right|^2\int\limits_{\Omega}\int\limits_{\mathrm{crystal}}\frac{\psi_{n\boldsymbol{k}}^{\sigma*}(\boldsymbol{r}')\psi_{n'\boldsymbol{k}'}^{\sigma}(\boldsymbol{r}')\psi_{n'\boldsymbol{k}'}^{\sigma*}(\boldsymbol{r}'')\psi_{n\boldsymbol{k}}^{\sigma}(\boldsymbol{r}'')}{|\boldsymbol{r}'-\boldsymbol{r}''|}d^3r'd^3r'', \tag{S11}$$

$$v_{\mathrm{x},\sigma}^{\mathrm{KLI,2,vc}}(\boldsymbol{r}) = \frac{1}{\rho_\sigma(\boldsymbol{r})}\sum_{n,\boldsymbol{k}}\sum_{\alpha}^{\mathrm{cell}}\sum_{n_c,\ell_c,m_c}w_{n\boldsymbol{k}}^{\sigma}\left|\psi_{n\boldsymbol{k}}^{\sigma}(\boldsymbol{r})\right|^2\int\limits_{S_\alpha}\int\limits_{S_\alpha}\frac{\psi_{n\boldsymbol{k}}^{\sigma*}(\boldsymbol{r}')\psi_{n_c\ell_cm_c}^{\alpha\sigma}(\boldsymbol{r}')\psi_{n_c\ell_cm_c}^{\alpha\sigma*}(\boldsymbol{r}'')\psi_{n\boldsymbol{k}}^{\sigma}(\boldsymbol{r}'')}{|\boldsymbol{r}'-\boldsymbol{r}''|}d^3r'd^3r'', \tag{S12}$$

$$v_{\mathrm{x},\sigma}^{\mathrm{KLI,2,cv}}(\boldsymbol{r}) = \frac{1}{\rho_\sigma(\boldsymbol{r})}\sum_{\alpha}^{\mathrm{cell}}\sum_{n_c,\ell_c,m_c}\sum_{n,\boldsymbol{k}}w_{n\boldsymbol{k}}^{\sigma}\left|\psi_{n_c\ell_cm_c}^{\alpha\sigma}(\boldsymbol{r})\right|^2\int\limits_{S_\alpha}\int\limits_{S_\alpha}\frac{\psi_{n_c\ell_cm_c}^{\alpha\sigma*}(\boldsymbol{r}')\psi_{n\boldsymbol{k}}^{\sigma}(\boldsymbol{r}')\psi_{n\boldsymbol{k}}^{\sigma*}(\boldsymbol{r}'')\psi_{n_c\ell_cm_c}^{\alpha\sigma}(\boldsymbol{r}'')}{|\boldsymbol{r}'-\boldsymbol{r}''|}d^3r'd^3r'', \tag{S13}$$

$$v_{\mathrm{x},\sigma}^{\mathrm{KLI,2,cc}}(\boldsymbol{r}) = \frac{1}{\rho_\sigma(\boldsymbol{r})}\sum_{\alpha}^{\mathrm{cell}}\sum_{n_c,\ell_c,m_c}\sum_{n_c',\ell_c',m_c'}\left|\psi_{n_c\ell_cm_c}^{\alpha\sigma}(\boldsymbol{r})\right|^2\int\limits_{S_\alpha}\int\limits_{S_\alpha}\frac{\psi_{n_c\ell_cm_c}^{\alpha\sigma*}(\boldsymbol{r}')\psi_{n_c'\ell_c'm_c'}^{\alpha\sigma}(\boldsymbol{r}')\psi_{n_c'\ell_c'm_c'}^{\alpha\sigma*}(\boldsymbol{r}'')\psi_{n_c\ell_cm_c}^{\alpha\sigma}(\boldsymbol{r}'')}{|\boldsymbol{r}'-\boldsymbol{r}''|}d^3r'd^3r''. \tag{S14}$$

The very detailed formulas for Eqs. (S3)-(S6) and (S11)-(S14) are similar as those presented in Ref. 4 for the Hartree-Fock method, where the pseudocharge method[5,6] combined with the technique proposed in Refs. 7 and 8 to treat the Coulomb singularity has been used.

## III. DETAILED RESULTS

Tables S2 and S3 show the errors in the EXX total energy and fundamental band gap, respectively.

---


1 O. K. Andersen, Phys. Rev. B **12**, 3060 (1975).
2 D. J. Singh and L. Nordström, *Planewaves, Pseudopotentials and the LAPW Method, 2nd ed.* (Springer, Berlin, 2006).
3 S. Blügel and G. Bihlmayer, *Computational Nanoscience: Do it Yourself!* (Forschungszentrum Jülich GmbH, 2006) p. 85.
4 F. Tran and P. Blaha, Phys. Rev. B **83**, 235118 (2011).
5 M. Weinert, J. Math. Phys. **22**, 2433 (1981).
6 S. Massidda, M. Posternak, and A. Baldereschi, Phys. Rev. B **48**, 5058 (1993).
7 G. Onida, L. Reining, R. W. Godby, R. Del Sole, and W. Andreoni, Phys. Rev. Lett. **75**, 818 (1995).
8 J. Spencer and A. Alavi, Phys. Rev. B **77**, 193110 (2008).

TABLE S2. EXX total energy calculated with orbitals generated from various exchange potentials. The values for the approximate potentials are the differences with respect to the values with the EXX-OEP orbitals. All values are in Ry/cell.

| Solid | EXX-OEP | EXX-KLI | LDA | PBE | EV93 | AK13 | gBJ |
|---|---|---|---|---|---|---|---|
| Ne | -257.378 | -0.001 | 0.037 | 0.026 | 0.020 | 0.014 | 0.000 |
| C | -151.592 | 0.004 | 0.042 | 0.027 | 0.017 | 0.029 | 0.003 |
| Si | -1158.353 | 0.007 | 0.078 | 0.040 | 0.015 | 0.027 | 0.000 |
| Ge | -8390.316 | 0.001 | 0.165 | 0.105 | 0.040 | 0.041 | 0.005 |
| BN | -158.623 | 0.002 | 0.047 | 0.027 | 0.015 | 0.023 | 0.002 |
| LiH | -16.126 | 0.002 | 0.021 | 0.007 | 0.008 | 0.036 | 0.001 |
| LiF | -214.363 | 0.001 | 0.059 | 0.028 | 0.011 | 0.028 | 0.003 |
| LiCl | -937.138 | -0.001 | 0.050 | 0.018 | 0.006 | 0.050 | -0.002 |
| BeO | -359.132 | 0.005 | 0.116 | 0.057 | 0.024 | 0.033 | 0.006 |
| MgO | -550.130 | 0.000 | 0.079 | 0.037 | 0.010 | 0.014 | 0.001 |
| BaO | -16422.319 | -0.007 | 0.117 | 0.051 | 0.016 | 0.036 | 0.009 |
| MnO | -4930.491 | 0.004 | 0.439 | 0.296 | 0.178 | 0.145 | 0.116 |
| NiO | -6377.727 | 0.180 | 0.896 | 0.592 | 0.404 | 0.304 | 0.257 |
| $Cu_2O$ | -13527.774 | 0.036 | 0.654 | 0.428 | 0.279 | 0.225 | 0.180 |
| ZnO | -7478.592 | 0.028 | 0.344 | 0.211 | 0.103 | 0.073 | 0.039 |
| $CeO_2$ | -18023.556 | 0.018 | 0.344 | 0.276 | 0.239 | 0.275 | 0.255 |

TABLE S3. Fundamental band gap (in eV) calculated with EXX-OEP and various approximate exchange potentials.

| Solid | EXX-OEP | EXX-KLI | LDA | PBE | EV93 | AK13 | gBJ |
|---|---|---|---|---|---|---|---|
| Ne | 14.73 | 14.37 | 10.80 | 11.00 | 10.72 | 20.07 | 15.40 |
| C | 4.57 | 4.21 | 4.00 | 4.46 | 4.60 | 4.78 | 4.44 |
| Si | 1.17 | 0.69 | 0.35 | 0.80 | 1.12 | 1.60 | 0.97 |
| Ge | 0.91 | 0.32 | 0.00 | 0.00 | 0.46 | 0.00 | 0.57 |
| BN | 5.43 | 4.92 | 4.20 | 4.89 | 5.25 | 5.68 | 5.03 |
| LiH | 4.04 | 3.50 | 2.52 | 3.52 | 4.26 | 6.16 | 3.98 |
| LiF | 11.16 | 10.61 | 8.71 | 9.41 | 10.16 | 12.59 | 10.42 |
| LiCl | 7.34 | 6.83 | 5.88 | 6.63 | 7.60 | 9.80 | 7.30 |
| BeO | 9.13 | 8.58 | 7.41 | 8.05 | 8.62 | 9.40 | 8.52 |
| MgO | 6.31 | 5.74 | 4.42 | 4.95 | 5.39 | 6.55 | 5.62 |
| BaO | 3.69 | 3.36 | 1.70 | 2.12 | 2.52 | 3.51 | 2.70 |
| MnO | 3.60 | 3.04 | 0.73 | 1.30 | 1.74 | 2.58 | 2.10 |
| NiO | 3.54 | 1.99 | 0.52 | 1.16 | 1.58 | 2.08 | 2.25 |
| $Cu_2O$ | 1.44 | 0.95 | 0.50 | 0.66 | 0.72 | 0.85 | 0.69 |
| ZnO | 2.89 | 2.08 | 0.53 | 0.94 | 1.39 | 2.10 | 1.69 |
| $CeO_2$ | 3.74 | 3.18 | 2.03 | 2.05 | 2.11 | 2.16 | 2.02 |
